# Supplementary material for: Fermion Pair Dynamics in Open Quantum Systems
Source: arXiv:2104.03195 source file (2021-04-07)
Supplement: Supplementary file 1 [file supplemental_material.pdf]

# Supplemental Material for "Fermion pair dynamics in open quantum systems"

S.M. Wang (王思敏)[1,2] and W. Nazarewicz[3]

[1] *FRIB Laboratory, Michigan State University, East Lansing, Michigan 48824, USA*
[2] *School of Physics, and State Key Laboratory of Nuclear Physics and Technology, Peking University, Beijing 100871, China*
[3] *Department of Physics and Astronomy and FRIB Laboratory, Michigan State University, East Lansing, Michigan 48824, USA*

This supplemental material contains:

- Supplemental discussions
- Supplemental figures
- Supplemental videos

## SUPPLEMENTAL DISCUSSIONS

### Jacobi coordinates

A two-nucleon emitter can be viewed as a three-body system: a core ($c$) representing the daughter nucleus and two emitted nucleons ($n_1$ and $n_2$). The $i$-th cluster ($i = c, n_1, n_2$) has the position vector $\boldsymbol{r}_i$ and linear momentum $\boldsymbol{k}_i$. In order to describe three-body asymptotics and to eliminate the spurious center-of-mass (c.m.) motion, it is convenient to adopt the relative (Jacobi) coordinates:

$$\begin{aligned} \boldsymbol{x} &= \sqrt{\mu_x}(\boldsymbol{r}_{i_1} - \boldsymbol{r}_{i_2}), \\ \boldsymbol{y} &= \sqrt{\mu_y}\left(\frac{A_{i_1}\boldsymbol{r}_{i_1} + A_{i_2}\boldsymbol{r}_{i_2}}{A_{i_1} + A_{i_2}} - \boldsymbol{r}_{i_3}\right), \end{aligned} \tag{S1}$$

where $i_1 = n_2, i_2 = c, i_3 = n_1$ for Y-coordinates and $i_1 = n_1, i_2 = n_2, i_3 = c$ for T-coordinates, see Figs. 1 and S1. In Eq. (S1) $A_i$ is the $i$-th cluster mass number, and $\mu_x = \frac{A_{i_1}A_{i_2}}{A_{i_1}+A_{i_2}}$ and $\mu_y = \frac{(A_{i_1}+A_{i_2})A_{i_3}}{A_{i_1}+A_{i_2}+A_{i_3}}$ are the reduced masses associated with $\boldsymbol{x}$ and $\boldsymbol{y}$, respectively. In practice, it is convenient to introduce the hyperradius $\rho = \sqrt{x^2 + y^2}$, which is transformation-invariant among different sets of Jacobi coordinates.

Since the experimental measurements are done in the momentum space, one defines the relative momenta:

$$\begin{aligned} \boldsymbol{k}_x &= \mu_x\left(\frac{\boldsymbol{k}_{i_1}}{A_{i_1}} - \frac{\boldsymbol{k}_{i_2}}{A_{i_2}}\right), \\ \boldsymbol{k}_y &= \mu_y\left(\frac{\boldsymbol{k}_{i_1} + \boldsymbol{k}_{i_2}}{A_{i_1} + A_{i_2}} - \frac{\boldsymbol{k}_{i_3}}{A_{i_3}}\right). \end{aligned} \tag{S2}$$

Since there is no c.m. motion, it is easy to notice that $\sum_i \boldsymbol{k}_i = 0$, and $\boldsymbol{k}_y$ is in the opposite direction of $\boldsymbol{k}_{i_3}$. $\theta_k$ and $\theta'_k$ are the opening angles of ($\boldsymbol{k}_x$, $\boldsymbol{k}_y$) in Y- and T-Jacobi coordinates, respectively (see Figs. 1 and S1). The kinetic energy of the relative motion of the emitted nucleons is given by $E_{pp/nn} = \frac{\hbar^2 k_x^2}{2\mu_x}$ and $E_{cp/cn}$ is that of the core-nucleon pair. To study the nucleon-nucleon correlation and the structural information about the mother nucleus, in this work, we divide them into two groups: (Cor1) correlations in $E_{pp/nn}$ and Y-type $\theta_k$; (Cor2) correlations in $E_{cp/cn}$ and T-type $\theta'_k$. Finally, the total momentum $k$ is defined as $\sqrt{\frac{k_x^2}{\mu_x} + \frac{k_y^2}{\mu_y}}$, which at late times approaches the limit $\frac{\sqrt{2mQ_{2p/2n}}}{\hbar}$, where $Q_{2p/2n}$ is the two-nucleon decay energy given by the binding energy difference of parent and daughter nuclei. For the excellent discussion of in Jacobi coordinates in the context of two-nucleon decays, see Refs. [1, 2].

### Interplay between initial-state and final-state interactions

Since the initial-state correlations are largely lost in the presence of Coulomb (final-state) interaction, one may be curious about whether some fingerprints of the initial correlations can still manifest themselves in the asymptotic observables, and what kind of role the initial-state interaction plays in the two-nucleon decay process. To address these questions, we studied the interplay between the initial-state and final-state interactions by adjusting the strength of the nucleon-nucleon (initial-state) interaction. Figure 3 illustrates how the $V_{pp}$ strength affects $pp$ correlations in the $2p$ decay of $^6$Be. When $V_{pp}$ is increased by 50% relative to the standard value, the weight of the $(K, \ell_x, \ell_y, S)$ = (0,0,0,0) Jacobi-coordinate configuration in the initial wave function grows from 7% to 23%. The resulting decay width ($\Gamma_{2p}$ = 442 keV) becomes more than five times larger as compared to the value obtained with the standard strength. As seen in Fig. S2 and related Supplemental Videos, increasing $V_{pp}$ causes a transition to the diproton decay, with the $pp$ wave function being dominated by the (0,0,0,0) $s$-wave configuration at late times. The stronger initial-state interaction results in a more uniform $pp$ energy distribution, shifted towards lower values of $E_{pp}$. The transition towards the diproton decay with stronger $V_{pp}$ is aided by the increased odd-even binding energy staggering, which reduces the amplitude of the one-proton decay branch. With the initial-state interaction reduced, the cigarlike branch becomes very significant and the $p$-wave configuration (2,1,1,0) becomes dominant. As seen in Fig. 3, at low values of $V_{pp}$, the energy correlation has two maxima: one at the low relative momenta of the emitted protons and another one at large relative momenta, which is consistent with the pattern seen in Fig. S2.

In the case of the $^6$He$'$, the initial-state interaction has similar effects on the energy correlation (see Fig. 3) as for $^6$Be. The angular $nn$ correlation becomes fairly uniform as $V_{nn}$ increases. This is due to the reason that a strong $V_{nn}$ can result in a fairly preserved dineutron structure and the opening angle of the emitted neutrons is rather arbitrary.

Figure S3 shows nucleon-nucleon correlations C2 in in Jacobi-T coordinates. Unlike in the case C1 shown in Fig. 3, here the correlations are not sensitive to the strength of initial-state interaction.

### Approximate decay law

To understand the behavior of two-nucleon decay, we arbitrarily divide the initial wave function $\Psi_0 \equiv \Psi_0^{J\pi}$ into an internal part $\Psi_0^{\rm int}$ and an asymptotic part $\Psi_0^{\rm ext}$:

$$\Psi_0 = \Psi_0^{\rm int} + \Psi_0^{\rm ext}. \tag{S3}$$

The initial wave function obtained with the complex-energy GCC method [3] is projected into the real-energy Hilbert space through the Fourier–Bessel series expansion. As a result, the internal wave function $\Psi_0^{\rm int}$ is well represented by the internally-localized GCC Gamow state of the complex energy $\tilde{E}_0$. However, in the asymptotic region, the purely outgoing wave function – proportional to the Coulomb wave function in the complex-momentum plane – becomes reduced to a wave packet of scattering states [4]. Therefore, according to the residue theorem, in the asymptotic region $\Psi_0^{\rm ext}$ can be formally expressed as:

$$\Psi_0^{\rm ext} = \int \frac{a(E)}{E - \tilde{E}_0} \, |E\rangle \, {\rm d}E, \tag{S4}$$

where $a(E)$ is the energy-dependent amplitude peaked around $E_0 = {\rm Re}(\tilde{E}_0)$, and $|E\rangle$ is the free three-body wave function with a real energy $E$ and total momentum $k$. The propagated wave function can be written as

$$\Psi(t) = e^{-i\frac{\hat{H}}{\hbar}t}\Psi_0^{\rm int} + e^{-i\frac{\hat{H}}{\hbar}t}\Psi_0^{\rm ext}. \tag{S5}$$

Since in the asymptotic region the nuclear interaction can be neglected, we approximate Eq. (S5) by

$$\Psi(t) \approx e^{-i\frac{\tilde{E}_0}{\hbar}t}\Psi_0 + \int a(E)\frac{e^{-i\frac{E}{\hbar}t} - e^{-i\frac{\tilde{E}_0}{\hbar}t}}{E - \tilde{E}_0}|E\rangle{\rm d}E, \tag{S6}$$

where the first term, limited to the internal region, exhibits an exponential decay with the width $\Gamma = -2\,{\rm Im}(\tilde{E}_0)$, while the second outgoing term converges to the resonance peak with a Breit-Wigner distribution $(E - \tilde{E}_0)^{-1}$ at late times [4]. This spatial diffusion during the decay process also corresponds to the gradually narrowing momentum distribution, in which only the components with energies around $E_0$ survive in the asymptotic region. The expression (S6) can also be derived by considering the difference between the self-adjoint Hamiltonian matrix and the complex-symmetric Hamiltonian matrix obtained by imposing the purely outgoing boundary condition as a perturbation.

The relation (S6) explains the decay pattern seen in Fig. 4. The first term of Eq. (S6) represents the initial wave function $\Psi_0$, which is localized inside the nucleus. For $^6$Be, the dominant (90%) component of $\Psi_0$ is $p^2$ with the $s^2$ component originating from the non-resonant continuum. Since the presence of positive and negative parity components is necessary for the appearance of di-nucleon correlations [5–8], large continuum space is essential for the formation of the diproton structure. As time evolves, the first term of Eq. (S6) decays exponentially and the outgoing flux is represented by the second term. At late times, the outgoing component has a narrowly distributed amplitude $a(E)$, which corresponds to the experimentally observed resonance [9]. The gradual configuration evolution and the associated interference pattern seen in Fig. 4 are governed by the factor $(e^{-i\frac{E}{\hbar}t} - e^{-i\frac{\tilde{E}_0}{\hbar}t})/(E - \tilde{E}_0)$ with a transition amplitude $a(E)$. Consequently, the frequency of the interference pattern is approximately given by the condition $\left[\frac{\hbar^2}{2m}k^2 - {\rm Re}(\tilde{E}_0)\right] t = \mathfrak{n}\pi\hbar$, where $\mathfrak{n} = 1, 3, 5 \cdots$.

**SUPPLEMENTAL FIGURES**

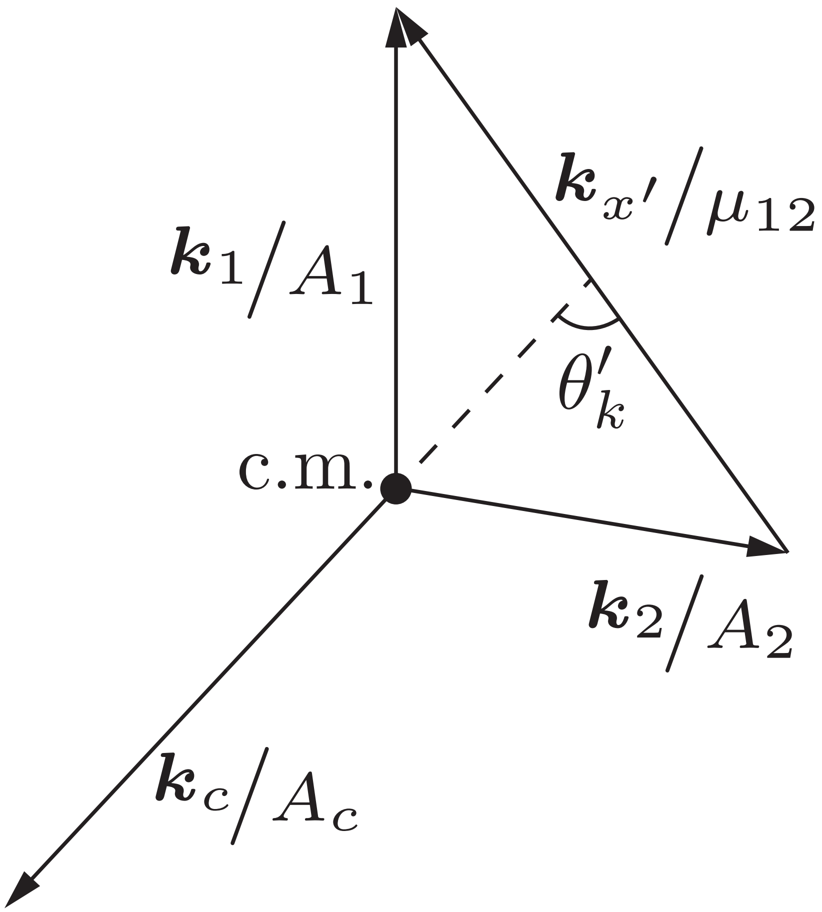


FIG. S1. The momentum scheme of Jacobi-T coordinates.

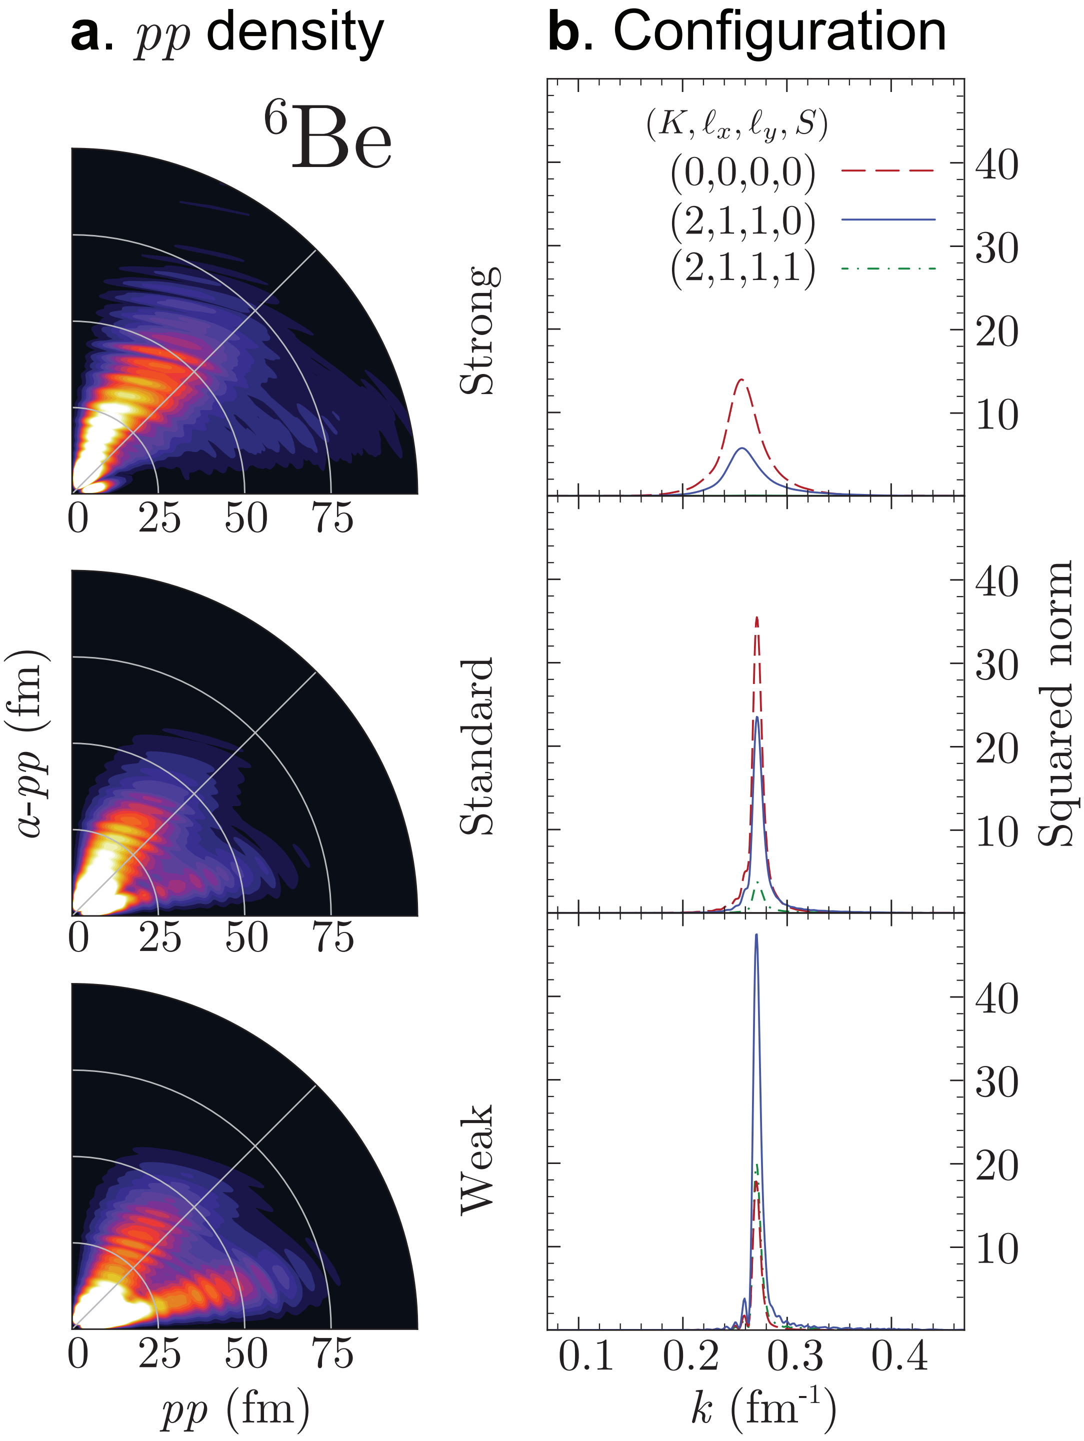


FIG. S2. Left: Density of two protons emitted from $^6$Be at early phase of tunnelling ($t = 0.7\,\mathrm{pm}/c$). Right: $2p$ wave function decomposition at late times ($t = 15\,\mathrm{pm}/c$). The results are shown for different strengths of Minnesota interaction: increased by 50% (top), standard (middle), and reduced by 50% (bottom). The densities are normalized to the total decay width. $k$ is the total momentum. The full width at half maximum of the momentum distribution is $4.4{\times}10^{-2}$, $6.8{\times}10^{-3}$, and $4.6{\times}10^{-3}$ (in fm$^{-1}$) for the strong, standard and weak nucleon-nucleon interaction, respectively. The correspond energy widths are 466, 73 and 50 keV.

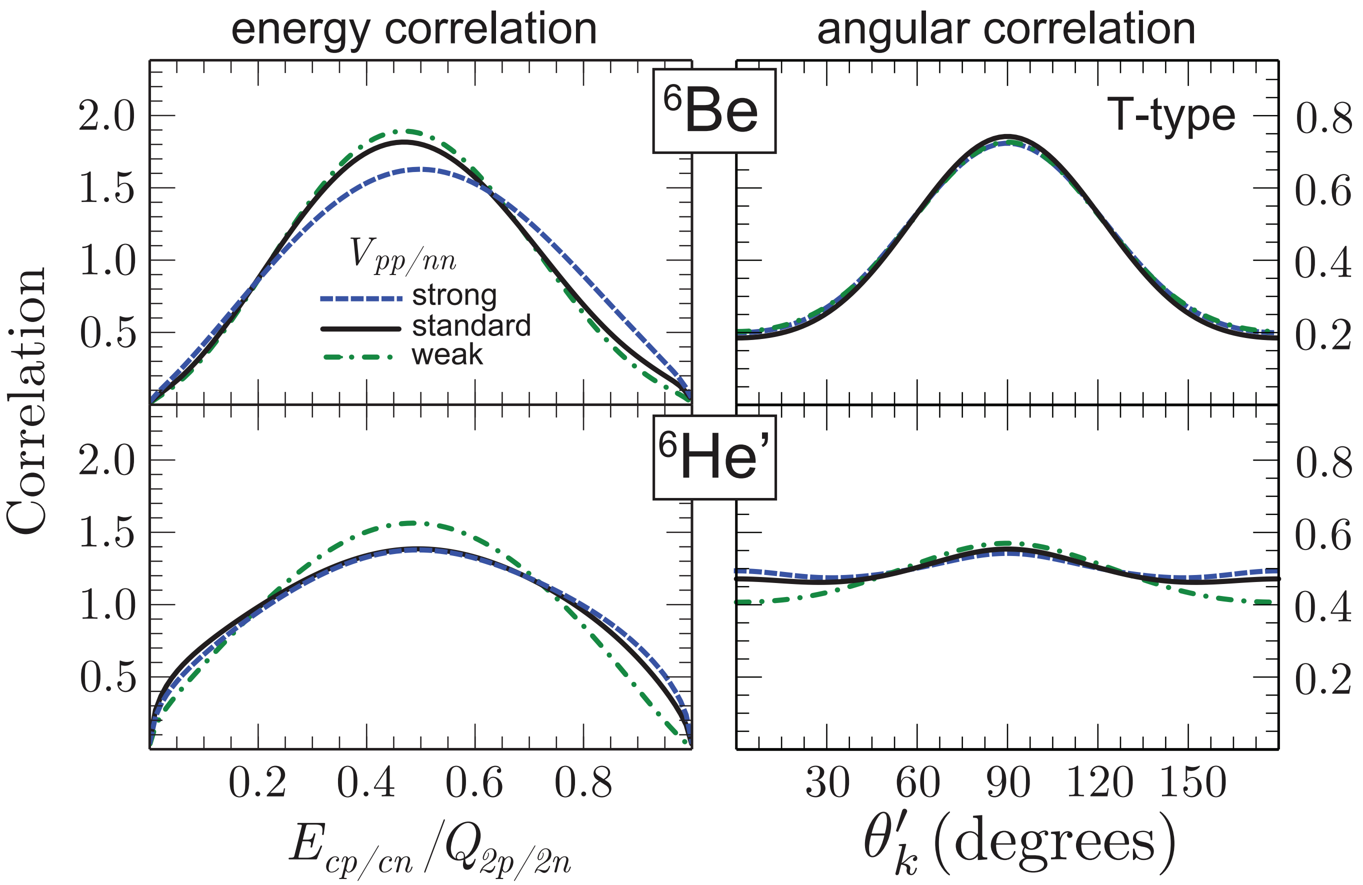


FIG. S3. Similar to Fig. 3, but in Jacobi-T coordinates. $\theta'_k$ is the opening angle between $\boldsymbol{k}_{x'}$ and $\boldsymbol{k}_c$ (see Fig. S1 for definitions), and $E_{cp/cn}$ is the kinetic energy of the relative motion of the core-nucleon pair.

## SUPPLEMENTAL VIDEOS

The supplemental videos (in a .mov format) show the time evolution of wave functions and two-nucleon densities for two-particle decay studied in this work. In the density plots, the outer turning line (line of outer turning points; estimated for the (0,0,0,0) $s$-wave configuration) is marked.

- Supplementary video 1: $2p$ decay from the ground state of $^6$Be in Jacobi T-coordinates.
- Supplementary video 2: $2n$ decay from the ground state of $^6$He$'$ in Jacobi T-coordinates.
- Supplementary video 3: Wave function evolution during the $2p$ decay of the ground state of $^6$Be.
- Supplementary video 4: Wave function evolution during the $2n$ decay of the ground state of $^6$He$'$.
- Supplementary video 5: Density evolution for the $2p$ decay of the ground state of $^6$Be for different strengths of pairing interaction $V_{pp}$.


[1] L.V. Grigorenko, T.D. Wiser, K. Miernik, R.J. Charity, M. Pfützner, A. Banu, C.R. Bingham, M. Ćwiok, I.G. Darby, W. Dominik, J.M. Elson, T. Ginter, R. Grzywacz, Z. Janas, M. Karny, A. Korgul, S.N. Liddick, K. Mercurio, M. Rajabali, K. Rykaczewski, R. Shane, L.G. Sobotka, A. Stolz, L. Trache, R.E. Tribble, A.H. Wuosmaa, and M.V. Zhukov, "Complete correlation studies of two-proton decays: $^6$Be and $^{45}$Fe," Phys. Lett. B **677**, 30–35 (2009).

[2] I. A. Egorova, R. J. Charity, L. V. Grigorenko, Z. Chajecki, D. Coupland, J. M. Elson, T. K. Ghosh, M. E. Howard, H. Iwasaki, M. Kilburn, Jenny Lee, W. G. Lynch, J. Manfredi, S. T. Marley, A. Sanetullaev, R. Shane, D. V. Shetty, L. G. Sobotka, M. B. Tsang, J. Winkelbauer, A. H. Wuosmaa, M. Youngs, and M. V. Zhukov, "Democratic decay of $^6$Be exposed by correlations," Phys. Rev. Lett. **109**, 202502 (2012).

[3] S. M. Wang, N. Michel, W. Nazarewicz, and F. R. Xu, "Structure and decays of nuclear three-body systems: The Gamow coupled-channel method in Jacobi coordinates," Phys. Rev. C **96**, 044307 (2017).

[4] A. I. Baz', Ya. B. Zel'dovich, and A. M. Perelomov, *Scattering, reactions and decay in nonrelativistic quantum mechanics* (Israel Program for Scientific Translation, Jerusalem, 1969).

[5] F. Catara, A. Insolia, E. Maglione, and A. Vitturi, "Relation between pairing correlations and two-particle space correlations," Phys. Rev. C **29**, 1091–1094 (1984).

[6] N. Pillet, N. Sandulescu, and P. Schuck, "Generic strong coupling behavior of Cooper pairs on the surface of superfluid nuclei," Phys. Rev. C **76**, 024310 (2007).

[7] K. Hagino and H. Sagawa, "Correlated two-neutron emission in the decay of the unbound nucleus $^{26}$O," Phys. Rev. C **89**, 014331 (2014).

[8] K. Fossez, J. Rotureau, N. Michel, and W. Nazarewicz, "Continuum effects in neutron-drip-line oxygen isotopes," Phys. Rev. C **96**, 024308 (2017).

[9] R. M. Id Betan and R. de la Madrid, "The Gamow-state description of the decay energy spectrum of neutron-unbound $^{25}$O," Nucl. Phys. A **970**, 398–410 (2018).
